# Supplementary material for: Semi-Supervised Action Recognition with Temporal Contrastive Learning
Source: arXiv:2102.02751 source file (2021-03-29)
Supplement: Supplementary file 1 [file supp_cont.tex]

\begin{table*}[!ht]
\centering
\resizebox{\columnwidth}{!}{%
\begin{tabular}{|c||c|}
\hline
 Page No. & Contents \\
\hline
\end{tabular}
}
% \caption{Comparison of our proposed approach with image-domain SSL baselines applied to Kinetics dataset using Resnet-18 backbone model. We report the Top-1 Clip accuracy values in each case.}
\label{tab:supp_con}
\end{table*}
